# Supplementary material for: Neural Embedding: Learning the Embedding of the Manifold of Physics Data
Source: arXiv:2208.05484 source file (2022-08-14)
Supplement: Supplementary file 1 [file appendix.tex]

Pictures of some jets
